# Supplementary material for: On Calibration of Scene-Text Recognition Models
Source: arXiv:2012.12643 source file (2020-12-23)
Supplement: Supplementary file 1 [file supplementary_for_review.tex]

\title{On Calibration of Scene-Text Recognition Models - Supplementary Material}

\maketitle
\input{latex/00_macros}

\input{latex/supplementary/910_suppl_intro}
\input{latex/supplementary/920_suppl_implementation}
\input{latex/supplementary/921_suppl_reliability}
\input{latex/supplementary/945_nll}
\input{latex/supplementary/960_varying_word_leng_and_temp}
\input{latex/supplementary/970_beam_search}
\clearpage
